# Supplementary material for: Bad-Metal Relaxation Dynamics in a Fermi Lattice Gas
Source: arXiv:1606.06669 ancillary file (2018-08-28)
Supplement: Supplementary file 1 [file SM3.pdf]

# Supplementary Information for “Bad Metal in a Fermi Lattice Gas”

W. Xu, W. McGehee,<sup>\*</sup> W. Morong, and B. DeMarco<sup>†</sup>

*Department of Physics, University of Illinois at  
Urbana-Champaign, Urbana, Illinois 61801, USA*

(Dated: May 28, 2017)

---

<sup>\*</sup>now at: Center for Nanoscale Science and Technology, National Institute of Standards and Technology,  
Gaithersburg, Maryland 20899, USA

<sup>†</sup>Electronic address: [bdemarco@illinois.edu](mailto:bdemarco@illinois.edu)

## I. EFFECTIVE CHEMICAL POTENTIAL AND TEMPERATURE

We use a relatively simple approach that leverages the adiabatic theorem of quantum mechanics and the absence of inter-particle interactions in the initially spin-polarized gas to estimate an effective chemical potential  $\tilde{\mu}$  and temperature  $\tilde{T}$ . These thermodynamic parameters are used to generate the semi-classical phase space distributions required by the weak scattering calculation and are needed to determine the density-weighted density. Our method involves calculating the occupation of single-particle eigenstates in the combined lattice and trap potential by assuming that the lattice turn-on satisfies the adiabatic theorem of quantum mechanics. These populations are then grouped and sorted by energy to form a distribution that is fit to a Fermi-Dirac (FD) profile.

Before turning on the optical lattice potential, the spin-polarized, non-interacting gas is trapped in a parabolic potential. The distribution of atoms in the single-particle eigenstates, characterized by three quantum numbers  $n_x$ ,  $n_y$ , and  $n_z$ , is therefore well described by a FD function  $f_{n_x, n_y, n_z} = 1/[e^{(\epsilon_{n_x, n_y, n_z} - \mu)/k_B T} + 1]$ , where  $\mu$  is the chemical potential,  $k_B$  is Boltzmann's constant, and  $T$  is the temperature. Here, the directions  $x$ ,  $y$ , and  $z$  correspond to the lattice axes. To determine the occupations  $f_{n_x, n_y, n_z}$  in the eigenstates for  $n_i = 1 \dots 300$ , we measure the number of atoms  $N$  and temperature of the gas using time-of-flight imaging. The chemical potential  $\mu$  is calculated by enforcing the constraint  $N = \sum_{n_x, n_y, n_z} f_{n_x, n_y, n_z}$ . We have checked that including more states does not significantly affect our results. We treat the trap as spherically symmetric, so that the energies are  $\epsilon_{n_x, n_y, n_z} = \hbar\tilde{\omega}(n_x + n_y + n_z)$ , where  $\tilde{\omega}$  is the geometric mean of the trap frequencies. We have also verified that taking into account the different trap frequencies does not affect the best estimate for  $\tilde{\mu}$  and  $\tilde{T}$ .

The single-particle eigenstates in the combined lattice-trap potential are also characterized by three quantum numbers [1, 2]. The lattice is turned on over 100 ms, which is much slower than all other timescales:  $\hbar/t \approx 0.5$  ms,  $\hbar/U \approx 55$   $\mu$ s, and  $\hbar/E_{bg} \approx 4$   $\mu$ s (at  $s = 7$ ), where  $E_{bg}$  is the bandgap. We therefore assume that the adiabatic theorem of quantum mechanics is satisfied, so that the distribution of particles in the lattice-trap eigenstates is unchanged, i.e.  $\tilde{f}_{n_x, n_y, n_z} = f_{n_x, n_y, n_z}$ . The corresponding eigenenergies are  $\tilde{E}_{n_x, n_y, n_z} = \tilde{E}_{n_x} + \tilde{E}_{n_y} + \tilde{E}_{n_z}$ , with

$$\tilde{E}_i = \begin{cases} \frac{\bar{\Omega}}{4} a_i(\alpha), & i \text{ even} \\ \frac{\bar{\Omega}}{4} b_{i+1}(\alpha), & i \text{ odd} \end{cases} \quad (1)$$

in the lattice-trap potential, where  $\bar{\Omega} = m\bar{\omega}^2 d^2/2$ ,  $\bar{\omega}$  is the geometric mean of the trap frequencies with the lattice light present,  $d$  is the lattice spacing,  $\alpha = 4t\bar{\Omega}$ , and  $a_i(\alpha)$  and  $b_{i+1}(\alpha)$  are the Mathieu characteristic values [1, 2]. We group and order the populations by energy to form a distribution  $\tilde{f}_{\tilde{\epsilon}_j} = \sum_{\tilde{E}_{n_x, n_y, n_z} = \tilde{\epsilon}_j} \tilde{f}_{n_x, n_y, n_z}$ , where  $j$  indexes the ordered, unique energies. We fit the distribution of occupations  $\tilde{f}_{\tilde{\epsilon}_j}$  to a FD function  $1/[e^{(\tilde{\epsilon}_j - \tilde{\mu})/k_B \tilde{T}} + 1]$  with an effective chemical potential  $\tilde{\mu}$  and temperature  $\tilde{T}$  as free parameters. The fit minimizes the sum of the squared difference at each  $\tilde{\epsilon}_j$  between  $\tilde{f}_{\tilde{\epsilon}_j}$  and the FD distribution.

Fig. S1 shows calculated  $\tilde{f}_{\tilde{\epsilon}_j}$  and fitted FD distributions for  $s = 4$ ,  $N = 26,400$ , and  $T/T_F = 0.22, 0.44$ , and  $1.16$ , which spans the full range of temperatures sampled in Fig. 4 in the main text. The results for the data in Fig. 3 of the main text for different  $s$  are similar to the lowest temperature point. The agreement between the computed  $\tilde{f}_{\tilde{\epsilon}_j}$  and the fitted distributions are excellent, except for the highest temperature points. At the highest temperatures, the procedure we use generates a distribution that underestimates the occupancy for the lowest and highest energy states (Fig. S1c). As we will discuss, despite this issue we find that our procedure provides a density distribution that closely matches the experiment, and thus the failure apparent at high temperature in Fig. S1 likely cannot explain the discrepancy in Fig. 3b in the main text.

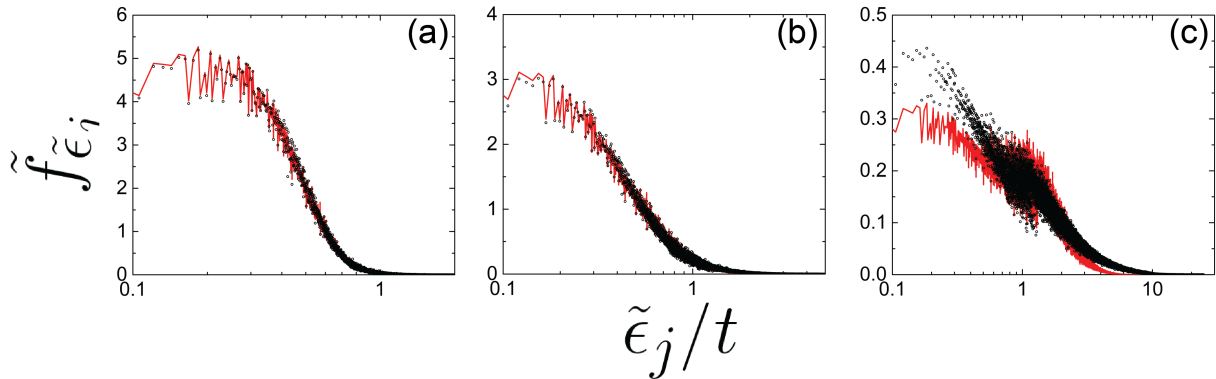

FIG. S1: Numerical data to determine effective chemical potentials and temperatures. The computed  $\tilde{f}_{\tilde{\epsilon}_j}$  is shown for  $s = 4$  and  $T/T_F = 0.22$  (a),  $0.44$  (b), and  $1.16$  (c) as open circles, and the fitted FD distribution is shown as a red line. A 20-point moving average filter is used to smooth the data, and approximately only one out of every 300 points are shown. Note the difference in vertical and horizontal scales.

In Fig. S2, we show the predicted  $\tilde{\mu}$  and  $\tilde{T}$  for the conditions of Fig. 3b in the main text for different values of  $T/T_F$  before the lattice is turned on. The effective degeneracy is approximately conserved as the lattice is turned on (i.e.,  $\tilde{T}/\tilde{T}_F \approx T/T_F$ ), and the effective chemical potential becomes negative for  $T/T_F \gtrsim 0.5$ , as for a trapped gas.

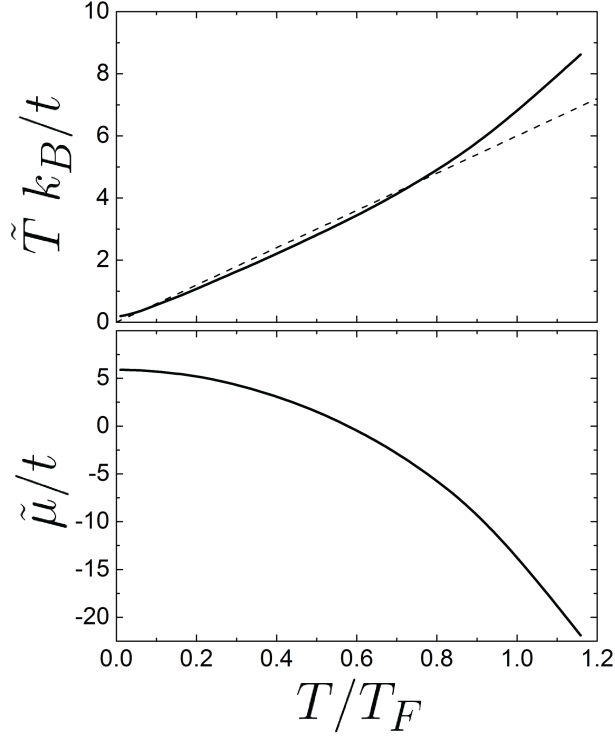

FIG. S2: The effective chemical potential and temperature scaled to the tunneling energy are shown as solid lines. The dashed line marks the condition for  $T/T_F$  to remain unchanged when the lattice is superimposed on the gas, where  $T_F \approx 6t/k_B$  in the lattice (according to a non-interacting calculation).

To verify our approach, we compare predicted and measured density profiles for a spin-polarized gas in the lattice-trap potential. Comparing measured quasimomentum profiles is complicated by the failure of bandmapping at the edge of the Brillouin zone (BZ) [2]. To measure the density profile, we first transfer approximately 90% of the atoms to the  $F = 7/2$  state using adiabatic rapid passage driven by a microwave-frequency magnetic field. This step is necessary to reduce the optical depth ( $OD$ ) of the gas. We then image the gas in situ. The images are angularly averaged (along ellipses that match the aspect ratio of the image) to produce a radial density profile. The measured ra-

dial profiles for  $s = 4$  and  $T/T_F = 0.25, 0.41$ , and  $1.1$  shown in Fig. S3 agree well with predicted profiles based on the estimated  $\tilde{\mu}$  and  $\tilde{T}$  and the semi-classical approximation. In the semi-classical approximation, the density  $n(\vec{r}) = \int d^3\vec{q} \tilde{\rho}(\vec{r}, \vec{q}, \tilde{\mu}, \tilde{T})/h^3$ , where  $\tilde{\rho}(\vec{r}, \vec{q}, \tilde{\mu}, \tilde{T}) = 1/\left[ e^{\left( m\tilde{\omega}^2 r^2/2 - 6t + 2t \sum_{j=x,y,z} \cos(\pi q_j/q_B) - \tilde{\mu} \right)/k_B \tilde{T}} + 1 \right]$  is the semi-classical phase space distribution in the combined lattice-trap potential.

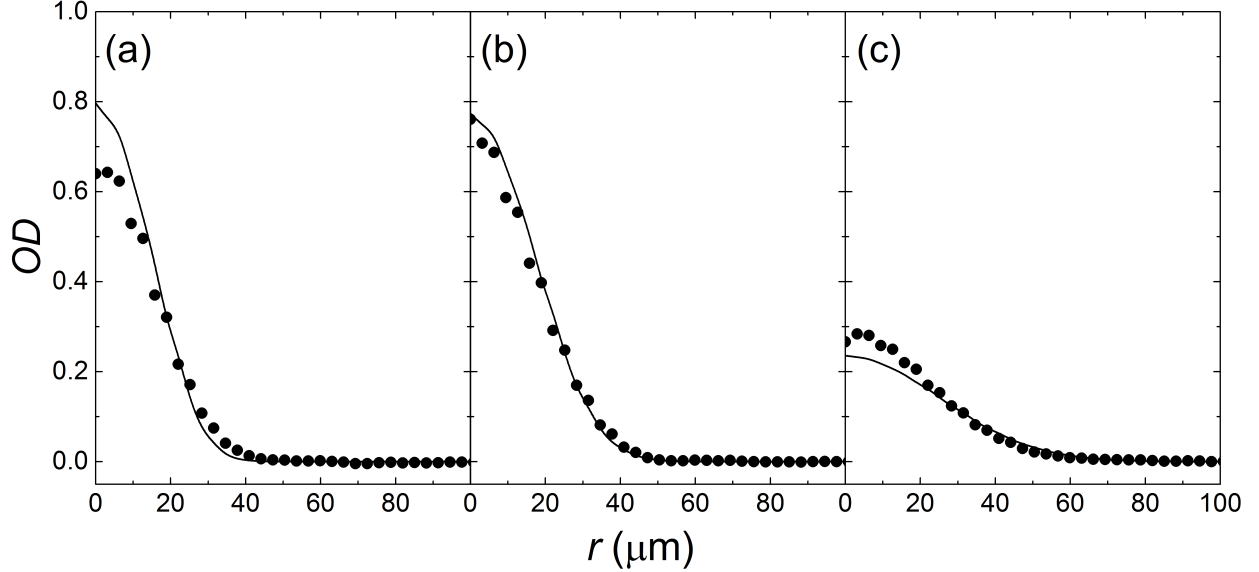

FIG. S3: Column-integrated radial density profiles for  $T/T_F = 0.25$  (a),  $0.41$  (b), and  $1.1$  (c) at  $s = 4$  shown as the measured optical depth (OD) in the trap. The measured profiles (solid circles) are created from averages of 3–4 images, and the prediction (solid line) is based on  $\tilde{\mu}$  and  $\tilde{T}$ . The predicted profile is scaled to match the number of atoms for each case:  $N=16500$  (a),  $22600$  (b), and  $15700$  (c). In this figure,  $r$  is a scaled radius that follows contours of constant  $OD$ .

For the weak scattering calculation of the transport lifetime, we assume that the semi-classical phase space distribution in the lattice before the Raman pulse is a FD distribution  $\xi \tilde{\rho}(\vec{r}, \vec{q}, \tilde{\mu}, \tilde{T})$  in the  $|\uparrow\rangle$  state, where  $\xi = N / \left[ \int d^3\vec{r} \int d^3\vec{q} \tilde{\rho}(\vec{r}, \vec{q}, \tilde{\mu}, \tilde{T})/h^3 \right]$  is a multiplicative factor used to fix the total atom number to the value in the experiment. This correction is necessary because the fitting procedure used to determine  $\tilde{\mu}$  and  $\tilde{T}$  is not constrained to correctly reproduce  $N$ . We approximate the Raman pulse as instantaneous, and use semi-classical distributions  $\tilde{\rho}_\uparrow(\vec{r}, \vec{q}) = \xi (1 - \gamma) \tilde{\rho}(\vec{r}, \vec{q}, \tilde{\mu}, \tilde{T})$  and  $\tilde{\rho}_\downarrow(\vec{r}, \vec{q}) = \xi \gamma \tilde{\rho}(\vec{r}, \vec{q} - \vec{\delta q}, \tilde{\mu}, \tilde{T})$  for the relaxation rate calculation. Here,  $\gamma \approx 0.35$  is the fraction of atoms transferred to the  $|\downarrow\rangle$  state by the Raman pulse. The shifted momentum  $\vec{q} - \vec{\delta q}$  of the  $|\downarrow\rangle$  particles is re-mapped

to the first BZ by subtracting reciprocal lattice vectors if it exceeds the first BZ boundary. Time-of-flight measurements indicate that the Raman lasers do not transfer atoms out of the first BZ, which is expected since the Raman Rabi rate is small compared with the bandgap.

There are several potential problems with our approach to creating a phase-space distribution. First, violations of adiabaticity and heating from scattering of lattice light will modify the distribution of atoms in the energy eigenstates. Also, Eq. 1 assumes that the principal axes of the trap are aligned with the lattice directions; a solution for the eigenstates without this constraint is unknown. In our experiment, these axes are not aligned, however. Finally, we assume that the trapping potential is spherically symmetric. In our experiment, the ratio of trap frequencies is 2.4:2.1:1. As the lattice is turned on, the overall trap potential becomes more spherically symmetric. Because the gas is collisionless, cross-dimensional thermalization is not possible [3], and the aspect ratio of the gas remains unchanged as the lattice is superimposed on the gas. We have verified this behavior for the images used to create Fig. S3. The two principal axes of the trap with trap frequencies in a 2.4:1 ratio lie within the imaging plane. We observe that the density profile of the gas before turning on the lattice has an aspect ratio of approximately 2 along these directions. This aspect ratio remains unchanged at  $s = 4$ , even though the ratio of trap frequencies along the imaging directions is 1.6:1. The good agreement apparent in Fig. S3 suggests that all of these complications are minor effects.

## II. TRANSPORT LIFETIME CALCULATION

We use a standard technique to calculate the transport lifetime rate based on Fermi's Golden Rule (FGR) that closely follows the approach used in Refs. 4 and 5. We allow for no free parameters in the calculation of the relaxation rate—experimentally measured values are used for all parameters. We use FGR to calculate the rate at which the Hubbard interaction term  $H_I = U \sum_i n_{i,\downarrow} n_{i,\uparrow}$  scatters particles between states of different quasimomentum. In this method,  $H_I$  is treated as a perturbation to the tight binding Hamiltonian  $-t \sum_{\langle ij \rangle, \sigma} (\hat{c}_{i\sigma}^\dagger \hat{c}_{j\sigma} + h.c.)$ . This approximation is only valid in the weakly interacting limit and is not satisfied in the experiment.

For this calculation we treat the  $|\uparrow\rangle$  gas as stationary (i.e., possessing no net quasimomentum). We use FGR to compute the time rate of change of the total quasimomentum of the  $|\downarrow\rangle$

component  $\langle\langle \partial(\vec{q}_\downarrow \cdot \hat{\delta k}) / \partial t \rangle\rangle$  along the direction of  $\vec{\delta k}$ , where  $\langle\langle \rangle\rangle$  represents a thermodynamic sum over all possible scattering events, and  $\hat{\delta k}$  is a unit vector along the Raman wavevector difference. We assume that the total quasimomentum  $\langle\vec{q}_\downarrow \cdot \hat{\delta k}\rangle = \int d^3\vec{r} \int d^3\vec{q} \tilde{\rho}_\downarrow(\vec{r}, \vec{q}) \vec{q} \cdot \hat{\delta k} / h^3$  of the  $|\downarrow\rangle$  gas decays exponentially, so that the transport lifetime is  $\frac{1}{\tau_t} = -\frac{1}{\langle\vec{q}_\downarrow \cdot \hat{\delta k}\rangle} \left\langle\left\langle \frac{\partial(\vec{q}_\downarrow \cdot \hat{\delta k})}{\partial t} \right\rangle\right\rangle$ .

We use dimensionless spatial and quasimomentum coordinates  $\vec{\mathcal{R}} = \vec{r}/d$  and  $\vec{\mathcal{Q}} = \pi\vec{q}/q_B$ , respectively, to carry out this calculation, such that  $\frac{1}{\tau_t} = -\frac{1}{\langle\vec{\mathcal{Q}}_\downarrow \cdot \hat{\delta k}\rangle} \left\langle\left\langle \frac{\partial(\vec{\mathcal{Q}}_\downarrow \cdot \hat{\delta k})}{\partial t} \right\rangle\right\rangle$ . FGR is used to calculate the time-rate-of-change of momentum as

$$\begin{aligned} \left\langle\left\langle \frac{\partial(\vec{\mathcal{Q}}_\downarrow \cdot \hat{\delta k})}{\partial t} \right\rangle\right\rangle &= \frac{1}{2} \frac{2\pi}{\hbar} \frac{U^2}{2t} \int d^3\vec{\mathcal{R}} \int \frac{d^3\vec{\mathcal{Q}}_{1\downarrow}}{(2\pi)^3} \int \frac{d^3\vec{\mathcal{Q}}_{2\uparrow}}{(2\pi)^3} \int \frac{d^3\vec{\mathcal{Q}}_{3\downarrow}}{(2\pi)^3} \tilde{\rho}_\downarrow(\vec{\mathcal{Q}}_{1\downarrow}, \vec{\mathcal{R}}) \tilde{\rho}_\uparrow(\vec{\mathcal{Q}}_{2\uparrow}, \vec{\mathcal{R}}) \times \\ &\quad [1 - \tilde{\rho}_\downarrow(\vec{\mathcal{Q}}_{3\downarrow}, \vec{\mathcal{R}})] [1 - \tilde{\rho}_\downarrow(\vec{\mathcal{Q}}_{4\uparrow}, \vec{\mathcal{R}})] (\vec{\mathcal{Q}}_{3\downarrow} - \vec{\mathcal{Q}}_{4\uparrow}) \cdot \hat{\delta k} \times \\ &\quad \delta[\tilde{\epsilon}(\vec{\mathcal{Q}}_{1\downarrow}) + \tilde{\epsilon}(\vec{\mathcal{Q}}_{2\uparrow}) - \tilde{\epsilon}(\vec{\mathcal{Q}}_{3\downarrow}) - \tilde{\epsilon}(\vec{\mathcal{Q}}_{4\uparrow})]. \end{aligned} \quad (2)$$

Eq. 2 integrates over scattering events between  $|\uparrow\rangle$  and  $|\downarrow\rangle$  atoms with initial momenta  $\vec{\mathcal{Q}}_{1\downarrow}$  and  $\vec{\mathcal{Q}}_{2\uparrow}$  and final momenta  $\vec{\mathcal{Q}}_{3\downarrow}$  and  $\vec{\mathcal{Q}}_{4\uparrow} = \vec{\mathcal{Q}}_{3\downarrow} - \vec{\mathcal{Q}}_{1\downarrow} - \vec{\mathcal{Q}}_{2\uparrow}$ . The value of  $\vec{\mathcal{Q}}_{4\uparrow}$  is mapped into the first BZ by subtracting reciprocal lattice vectors if it exceeds the first BZ boundary. The dimensionless tight-binding energies are  $\tilde{\epsilon}(\vec{\mathcal{Q}}) = 2(3 - \cos \mathcal{Q}_x - \cos \mathcal{Q}_y - \cos \mathcal{Q}_z)$ .

We evaluate Eq. 2 using Markov-chain Monte Carlo integration. The energy-conserving delta function is represented as a decaying exponential proportional to  $e^{-|\tilde{\epsilon}|/l}$ . We make  $l$  sufficiently small such that the error introduced by representing the delta function this way is smaller than the Monte Carlo integration uncertainty, which is approximately 1%. For Fig. 3a in the main text, we use the value of  $\tilde{\mu}$  and  $\tilde{T}$  averaged across the data to generate the theory curve, while for Fig. 3b, we use the average value of  $N$ .

### III. RELAXATION FOR SPIN-POLARIZED GAS

Because of the tight-binding dispersion, the gas in the lattice is not harmonic, and hence Kohn's theorem does not hold. Therefore, center-of-mass motion such as we excite will decay as individual atomic trajectories dephase. We experimentally probe and theoretically model this dephasing time to verify that the relaxation we measure is dominated by interaction-induced scattering between quasimomentum states. To measure the dephasing time, we apply an impulse to a spin-polarized gas trapped in the lattice. A force generated via a magnetic field gradient is applied to the atoms along the same direction as the Raman

wavevector difference. The strength of the force is tuned to transfer approximately the same momentum to the gas as the Raman excitation.

Sample measurements of the average quasimomentum of the gas for different hold times in the lattice after the impulse is applied are shown in Fig. S4 for  $T/T_F \approx 0.25$  (before the lattice is turned on) and  $N \approx 42000$ . We analyze the data in the same way as the main text and fit to Eq. 2 to determine a dephasing timescale  $\tau$ . These data approximately match the condition for the  $s = 4$  point in Fig. 3a and the lowest temperature point in Fig. 3b in the main text.

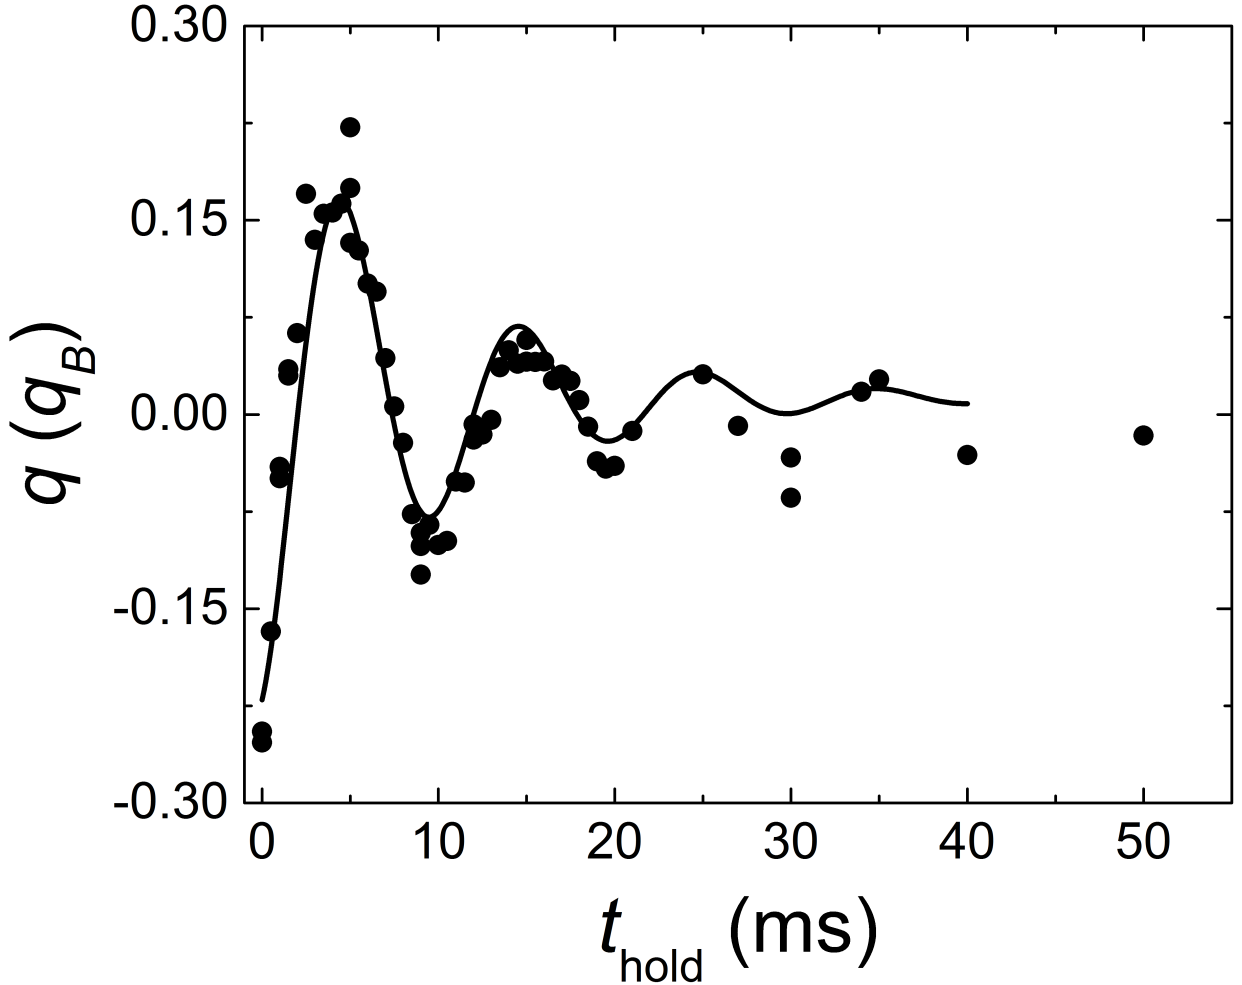

FIG. S4: Measured average quasimomentum  $q$  along the impulse direction for a spin-polarized gas in an  $s = 4$  lattice. For these data,  $N \approx 42000$  and  $T/T_F \approx 0.25$  in the trap before turning on the lattice. The solid line is a fit used to determine the dephasing time.

We simulate the dephasing time by propagating classical trajectories for a thermal dis-

tribution of initial quasimomenta subjected to the same impulse as in the experiment. For this simulation, we work in 1D, use 3000 particles, and propagate the position and quasimomentum of each particle according to  $dx/dt = \partial H/\partial q$  and  $dq/dt = -\partial H/\partial x$  with  $H = m\bar{\omega}^2 x^2/2 + 2t[1 - \cos(\pi q/q_B)]$ . We weight the quasimomentum of the particles by a FD distribution and determine for average quasimomentum for different propagation times. The results of a simulation for  $\tilde{\mu} = 4.5t/3$  and  $\tilde{T} = 1.3(t/k_B)/3$  (in the lattice) are shown in Fig. S5. We choose thermodynamic parameters a factor of three times smaller than the corresponding experimental points to account for the three times smaller bandwidth in 1D compared with 3D. With this adjustment, the parameters used for Fig. S5 match the experimental conditions for the lowest temperature point in Fig. 3b in the main text and those in Fig. S4. As with the experimental data, we determine a dephasing time by fitting the simulated data to Eq. 2.

A summary of the measured and simulated dephasing times is shown in Fig. S6 for different temperatures in an  $s = 4$  lattice. The data shown in Fig. 3a in the main text will behave similarly to the lowest temperature point. For comparison, the corresponding measured transport lifetimes from Fig. 3b in the main text are displayed. As expected, the dephasing time is smaller at higher temperature since a wider range of quasimomenta are present. The agreement between simulated and measured dephasing times for spin-polarized gases indicates that the simulation accurately describes the dephasing dynamics. The simulated dephasing times have much smaller uncertainties than the measurements and therefore are a useful benchmark for estimating the impact of dephasing on our measurements. The simulated dephasing time is at least 4 times longer than the measured transport lifetime. At high temperature, where the deviation from weak scattering theory is largest, the simulated dephasing time is 6 times longer than the measured transport lifetime. We conclude that dephasing has a minor impact on our measurements.

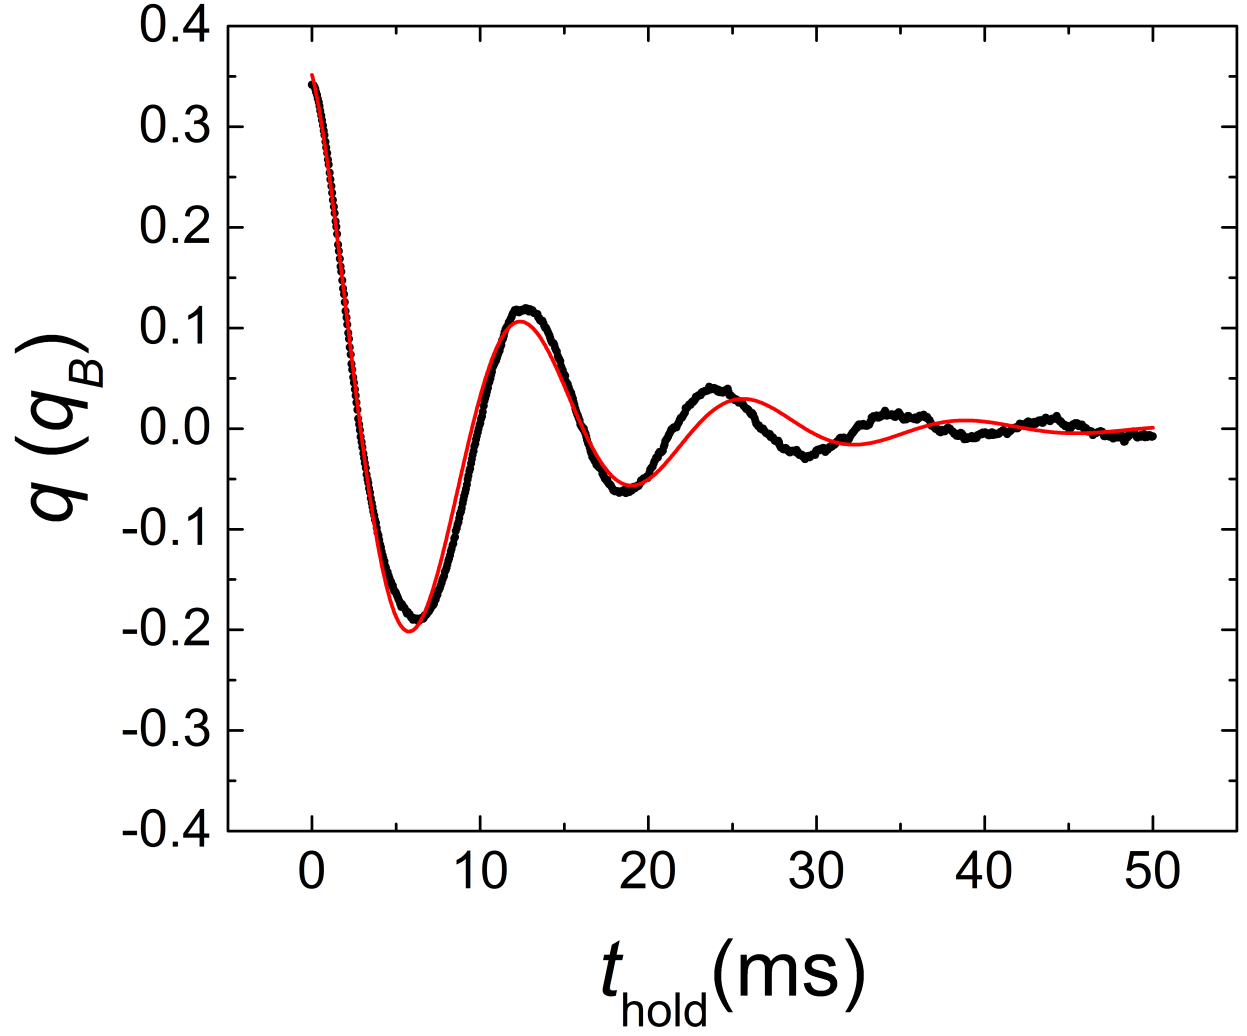

FIG. S5: Simulated average quasimomentum  $q$  along the impulse direction for a spin-polarized gas in an  $s = 4$  lattice. For this simulation,  $\tilde{T} = 1.3(t/k_B)/3$  and  $\tilde{\mu} = 4.5t/3$  in the lattice. The deviation of the fit at long times is a result of the anharmonicity of the lattice gas, which is not accounted for in the fit.

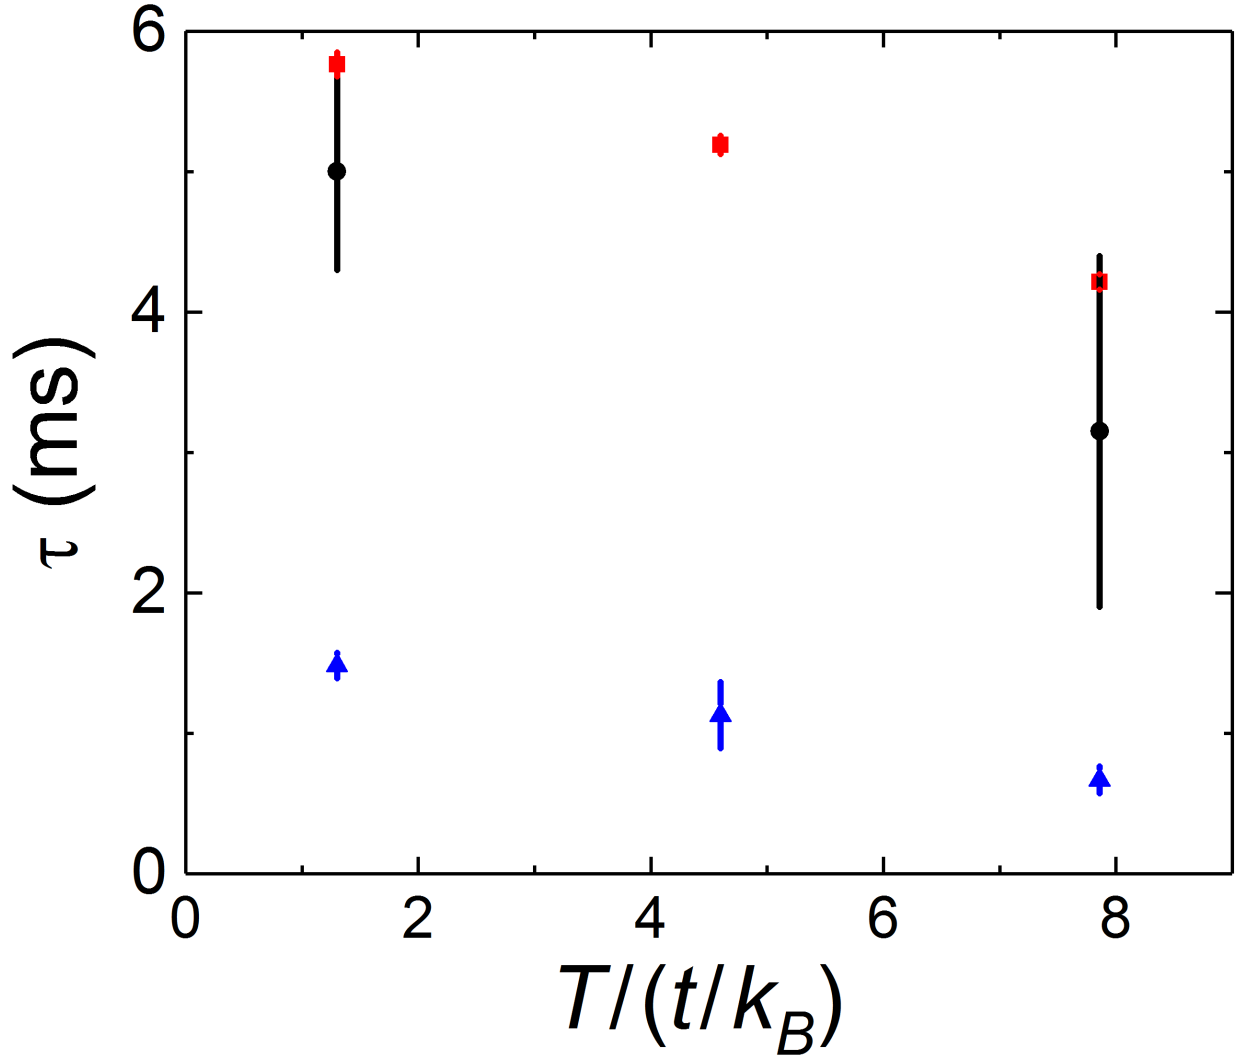

FIG. S6: Comparison of dephasing and transport lifetime  $\tau$  at different temperatures in an  $s = 4$  lattice. The dephasing time measured using a spin-polarized gas are shown using black circles, and the measured transport lifetime for a spin-mixed gas is shown using blue triangles. The simulated dephasing time is plotted using red squares. For the simulated time, the temperature is three times smaller than the value on the abscissa. The chemical potentials used in the simulation are  $4.5t/3$ ,  $-4.5t/3$ , and  $-18.2t/3$ . The error bars represent the uncertainty in the fit used to determine  $\tau$ .

#### IV. DMFT CALCULATION

Dynamical mean field theory maps a many-body lattice model to a local single-site problem, where the influence from adjacent sites is replaced by an effective coupling to an external bath [6]. We adapted the code provided in the Toolbox for Research on Interacting Quantum Systems (TRIQS) [7], which employs iterated perturbation theory to obtain the Green's functions for the Hubbard model with a Bethe lattice geometry and particle-hole symmetry. Despite the simplicity of this method, it is believed to give a qualitatively correct result and scalings for physical quantities [6, 8]. The conductivity  $\sigma(\omega)$  for a charged system under the bubble-pair approximation can be calculated as [9]:

$$\sigma(\omega) = \frac{\pi e^2}{\hbar} \int_{-\infty}^{\infty} d\epsilon \Psi(\epsilon) \int_{-\infty}^{\infty} d\omega' \frac{f(\omega') - f(\omega + \omega')}{\omega} A(\omega', \epsilon) A(\omega' + \omega, \epsilon), \quad (3)$$

where  $e$  is the charge of the carriers, the spectral function  $A(\omega, \epsilon) = -\text{Im} \left( \frac{1}{\omega + \mu - \Sigma(\omega) - \epsilon} \right) / \pi$ ,  $\Sigma(\omega)$  is the self-energy,  $\mu$  is the chemical potential, and  $f(\omega)$  is the Fermi-Dirac distribution.  $\Psi(\epsilon) = \sum_k \left( \frac{\partial \epsilon_k}{\partial k} \right)^2 \delta(\epsilon - \epsilon_k)$  is the transport density of states, and  $\epsilon_k$  is the energy of the state in the lattice. For the Bethe lattice,  $\Psi(\epsilon) = \Psi(0) [1 - (\epsilon/W)^2]^{3/2}$ , where  $W$  is the half-bandwidth.

In our DMFT calculation, the temperature and energies are in units of the half-bandwidth  $W$ , which is  $6t$  for our lattice. Fig. S7 shows the dependence of the dc resistivity  $\rho = 1/\sigma(0)$  (in arbitrary units) on the interaction strength at  $T/W = 0.248$ , which corresponds to the conditions for Fig. 3a in the main text. Within the interaction range that our measurements explored, the resistivity  $\rho$  follows a  $(U/W)^2$  scaling for  $U/W < 1$ . This dependence is consistent with Fermi-liquid theory. At higher  $U$ , a slight deviation from quadratic scaling is observed. For the range of temperature we sample, although the weight of quasiparticles at the Fermi energy decreases as  $U$  increases, a well-resolved peak in the vicinity of the Fermi level still exists (Fig. 4a in the main text), and the weight in the lower and higher Hubbard bands remains negligible.

Fig. S8 plots the dependence  $\rho$  on temperature at  $U/W = 0.383$ , corresponding to the conditions for Fig. 4b in the main text. At low  $T$  (i.e.,  $T/W < 0.1$ ), the resistivity shows a quadratic scaling of  $T$ , which is the prediction from Fermi-liquid theory. As  $T$  increases, a linear-dependence on temperature appears, indicating that the picture describing transport as coherent scattering among well-defined quasiparticles is invalid.

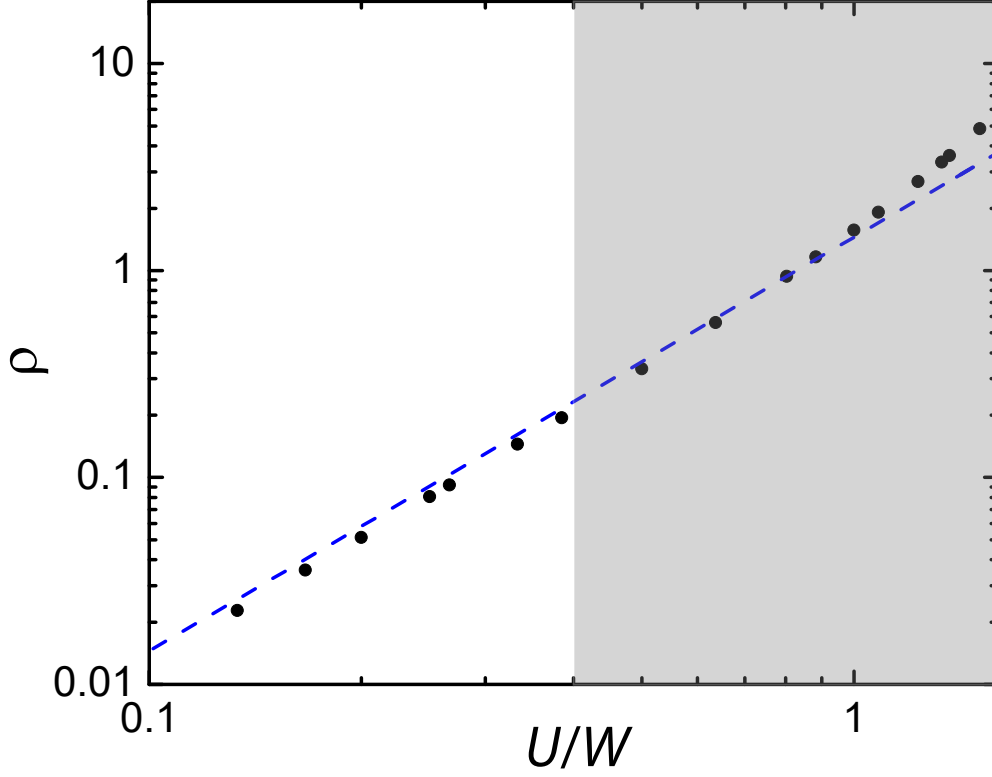

FIG. S7: Dependence of the resistivity on interaction strength with  $k_B T/W = 0.248$ , which corresponds to the averaged temperature for the relaxation time measurements shown in Fig.3(a). The blue dashed line is a fit to  $(U/W)^2$  for  $U/W < 1$ . The shaded region shows the area of this plot relevant to the experiment, which samples  $U/W = 0.4$ – $1.5$ .

Our DMFT calculation assumes particle-hole symmetry and half-filling. The experiment, however, involves an unequal number of  $|\downarrow\rangle$  and  $|\uparrow\rangle$  atoms and an inhomogeneous density profile. While the particle-hole asymmetry is known to modify the spectral function  $A(\omega)$  [10] and affect the absolute value of resistivity, more sophisticated DMFT calculations indicate that  $T$ -linear resistivity still appears within the temperature range we sample [11]. Other methods, such as quantum Monte Carlo calculations [12], also show the existence of  $T$ -linear scaling within a wide range of filling factors.

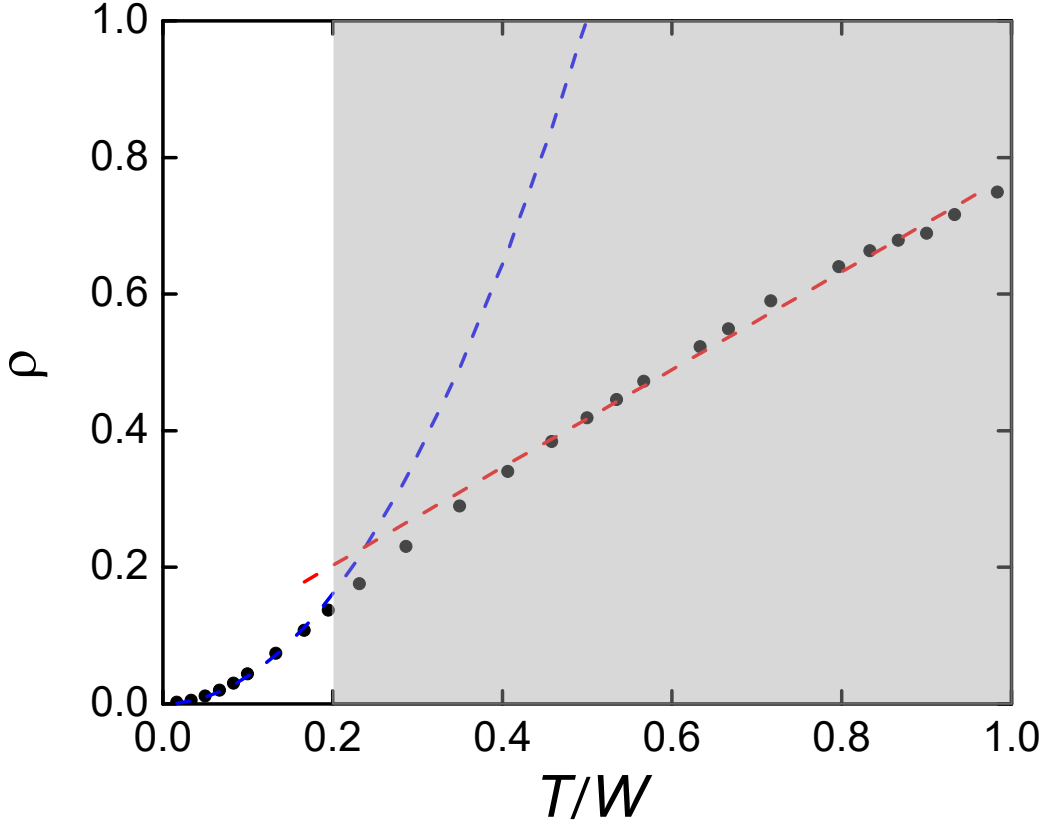

FIG. S8: Temperature dependence of resistivity at  $t/W = 0.383$ , corresponding to a lattice depth  $s = 4E_R$ . At very low temperature, the resistivity is proportional to  $T^2$  as expected in Fermi-liquid theory, suggesting coherent scattering between well-defined quasiparticles. As  $T$  increasing, a linear dependence on  $T$  appears, corresponds to the bad metal regime of transport. The blue dashed line is a fit to a quadratic function for  $T/W < 0.1$ , and the red dashed line is a linear fit for  $T/W > 0.1$ . The shaded region shows the area of this plot relevant to the experiment, which samples  $T/W = 0.2$ – $1.3$ .

## V. RESISTIVITY

A complication is that DMFT simulates a spatially uniform system, while our measurements are averaged over the inhomogeneous atomic density profile. We must therefore correct our measured  $\tau_t$  for this average.

For any process that generates resistivity through independent two-body scattering, with-

out losing generality, we can write  $1/\tau_t = n_s M$ , where  $M$  is an integral (over momenta) of scattering matrix elements that contribute to the decay of current, and  $n_s$  is the density of scatterers. The resistivity is proportional to  $m^*/\tau_t$ , where  $m^*$  is the effective mass. The challenge in determining resistivity for strongly correlated systems is evaluating  $M$ .

In our case,  $n_s = n_\uparrow(\vec{r})$ , which varies across the gas. Our measured transport lifetime is a weighted average  $M \int d^3r n_\uparrow(\vec{r}) n_\downarrow(\vec{r}) / N_\downarrow = M n_{dwd}$  over the  $|\downarrow\rangle$  density profile, which links our measurements with  $M$ . Here,  $n_{dwd}$  is the density-weighted density, and  $N_\downarrow$  is the number of atoms in the  $|\downarrow\rangle$  state. To compare with DMFT simulations, which involves a uniform system with fixed electron density, we therefore divide the measured  $\tau_t$  by  $n_{dwd}$ . In addition, since  $m^* \propto t$ , we absorb a factor of  $t$  into a dimensionless  $\tau_t / (\hbar/t)$ , and define the dimensionless resistivity  $\varrho = 1 / \frac{\tau_t}{\hbar/t} n_{dwd} d^3$ .

Our analysis of  $\varrho$  assumes that the thermally averaged relative speed between colliding partners is independent of temperature. We assume that the thermally averaged speed of the  $|\downarrow\rangle$  component is also fixed with respect to changes in temperature for our determination of  $\varrho_{\text{MIR}}$ . Variation in the thermally averaged speeds of the particles is suppressed because  $E_F \approx 6t$  and there is a maximum allowed speed in this single-band system. As shown in Fig. S9, the thermally averaged speeds are independent of temperature to an excellent approximation for our parameter regime.

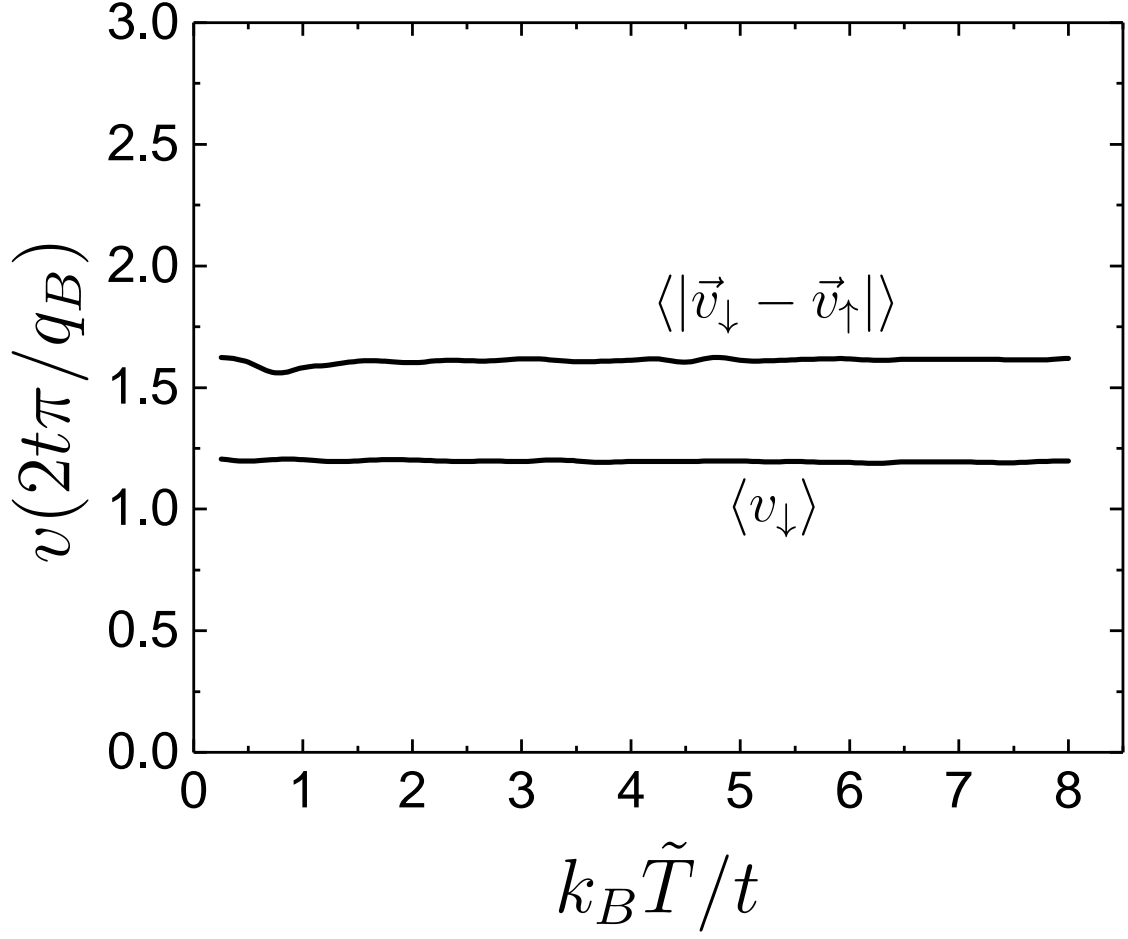

FIG. S9: The thermally averaged speed between colliding partners and for the  $|\downarrow\rangle$  component. These parameters are determined using  $\tilde{\mu}$  and  $\tilde{T}$ .

- 
- [1] A. M. Rey, G. Pupillo, C. W. Clark, and C. J. Williams, Phys. Rev. A **72**, 033616 (2005).
  - [2] D. McKay, M. White, and B. DeMarco, Phys. Rev. A **79**, 063605 (2009).
  - [3] B. DeMarco, J. L. Bohn, J. P. Burke, M. Holland, and D. S. Jin, Phys. Rev. Lett. **82**, 4208 (1999).
  - [4] D. Chen, C. Meldgin, and B. DeMarco, Phys. Rev. A **90**, 013602 (2014).
  - [5] D. C. McKay, C. Meldgin, D. Chen, and B. DeMarco, Phys. Rev. Lett. **111**, 063002 (2013).
  - [6] A. Georges, G. Kotliar, W. Krauth, and M. J. Rozenberg, Rev. Mod. Phys. **68**, 13 (1996).
  - [7] O. Parcollet, M. Ferrero, T. Ayrat, H. Hafermann, I. Krivenko, L. Messio, and P. Seth, Comput. Phys. Commun. **196**, 398 (2015).
  - [8] A. Georges and G. Kotliar, Phys. Rev. B **45**, 6479 (1992).
  - [9] N. Pakhira and R. H. McKenzie, Phys. Rev. B **91**, 075124 (2015).
  - [10] H. Kajueter and G. Kotliar, Phys. Rev. Lett. **77**, 131 (1996).
  - [11] X. Deng, J. Mravlje, R. Žitko, M. Ferrero, G. Kotliar, and A. Georges, Phys. Rev. Lett. **110**, 086401 (2013).
  - [12] M. Jarrell and T. Pruschke, Phys. Rev. B **49**, 1458 (1994).
